# Supplementary material for: Using dynamic circles and squares to visualize spatio-temporal variation
Source: arXiv:2211.05965 source file (2022-11-11)
Supplement: Supplementary file 1 [file survey_appendix_v2.pdf]

Section 1 of 9

# Geo-shape Visualization User Study

Form description

The Research - Purpose of Study

**Project title:** Geo-shape Visualization User Study

**Purpose of the Study:** We invite you to participate in our research study that aims to understand how we visualize shapes in general by comparing areas, lengths, and perimeters.

**Procedures:**
You will solve questions about squares vs circles and provide feedback.

**You are eligible if**:
- You have not participated in this study before.
- You are located in the U.S.
- You are at least 18 years old.
- You are using a laptop/desktop computer, or mobile device.
- You do not have color blindness or color vision deficiency.
- You are comfortable with reading/interpreting maps and size of shapes.

**How long will the study take**?
We expect this study to take around 5-10 minutes.

**What are your benefits**?
This research is not designed to benefit you personally.
We hope that, in the future, other people might benefit from this study through improved information visualization design.

**What are your risks**?
There are no known risks associated with participating in this research project.
We discuss confidentiality of your participation below.

[illegible]

*Your participation in this research is completely voluntary. You may choose not to take part at all. If you decide to participate in this research, you may stop participating at any time. If you decide not to participate in this study or if you stop participating at any time, you will not be penalized or lose any benefits to which you otherwise qualify.* If you withdraw prior to completing the study, you will not receive compensation.

Selecting "Yes" will indicate that you agree to participate and that

- You have read this consent form,
- You are eligible to participate in this study,
- You have had an opportunity to ask questions about your participation, and
- You voluntarily consent to participate.

Do you want to participate? *

- Yes
- No

After section 1 Continue to next section

Section 2 of 9

Worker ID

Description (optional)

Provide your worker ID *

Short answer text

After section 2 Continue to next section

Section 3 of 9

Diameter and Side Length Tasks

Using only the visual information on the maps, please estimate (by eye) the relative sizes of the **black dotted shapes**. Note: the values are arbitrary, so no outside information will be useful.

Definitions:

Diameter of Circle - a straight line that runs from one side of the circle to the other, passing through the center (basically the maximum width of the circle)
Side Length of Square - one side of the square

1. Ohio (D: OH)  has a black dotted circle with a **diameter** of 100. *

What is the **diameter** of Illinois (A: IL)'s black dotted circle?

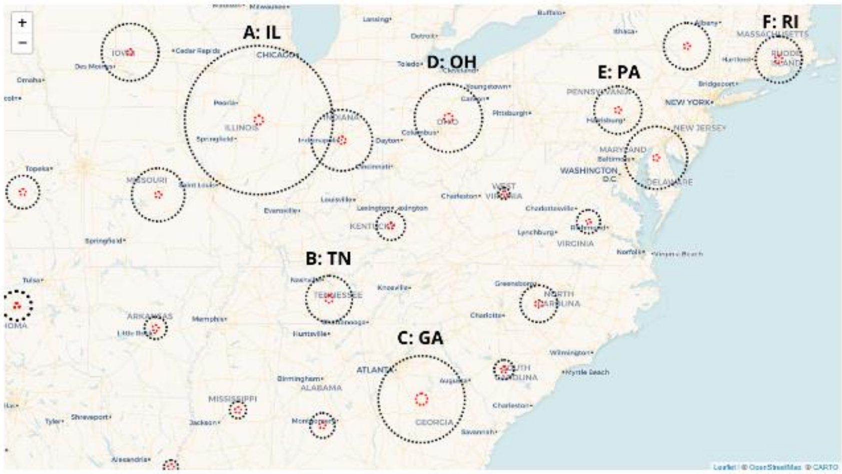


- 200
- 210
- 220
- 230

2. Tennessee (B: TN) has a black dotted circle with a **diameter** of 70. *

What is the **diameter** of Pennsylvania (E: PA)'s black dotted circle?

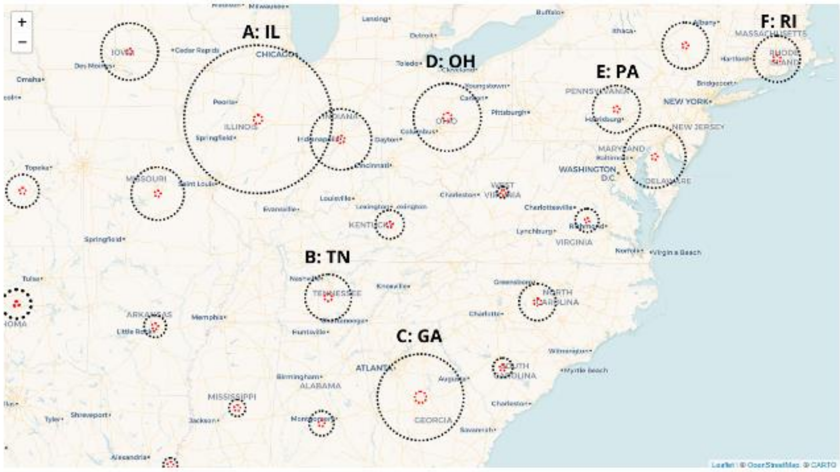


- 60
- 70
- 80
- 90

3. Ukraine has a black dotted square with a **side length** of 60. *

What is the **side length** of United Kingdom's black dotted square?

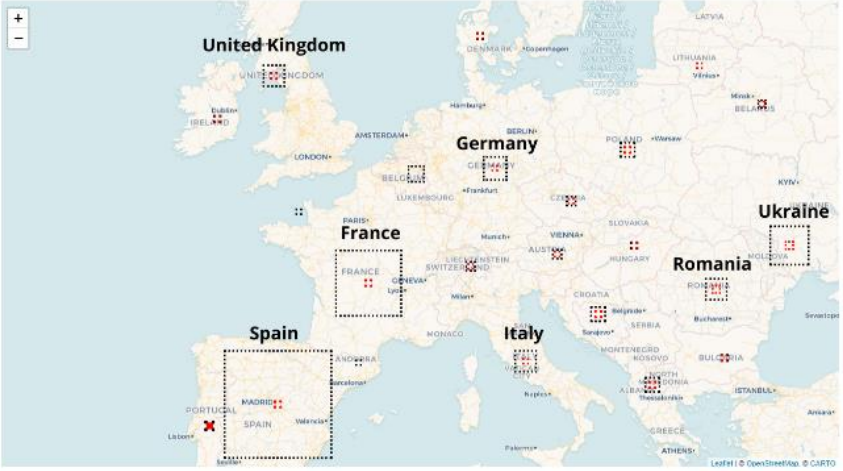


- 20
- 30
- 40
- 50

4. Using the statistics written in the image, approximately how many **deaths** does Georgia have? *

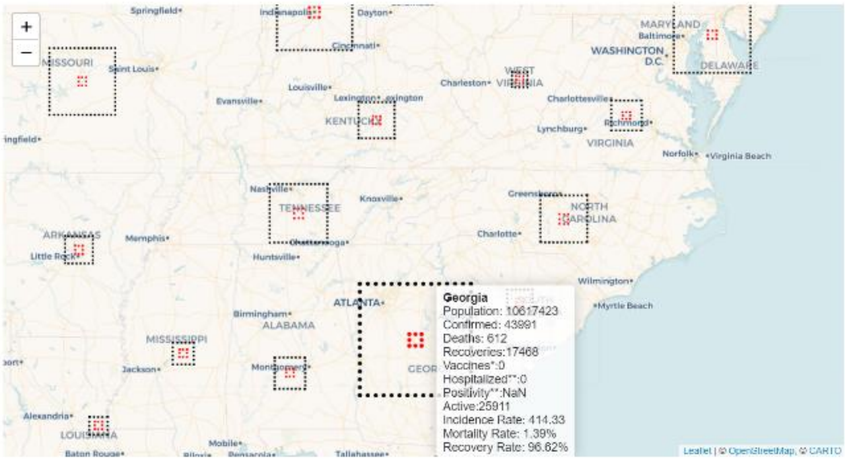


- 900
- 100
- 600
- 700

5. France has a black dotted square with a **side length** of 100. *

What is the **side length** of Spain's black dotted square?

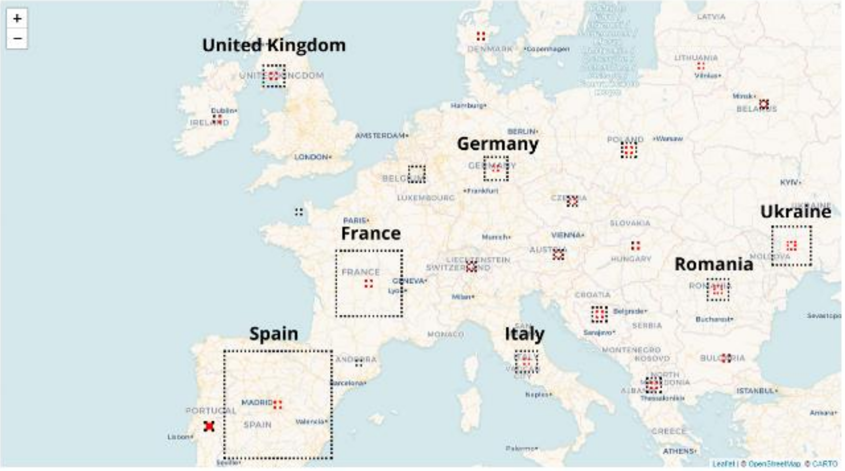


- 120
- 140
- 160
- 180

6. Wisconsin (WI) has a black dotted circle with a **diameter** of 150 (as seen on the left image). *

What is the **diameter** of Wisconsin (WI)'s black dotted circle on the right?

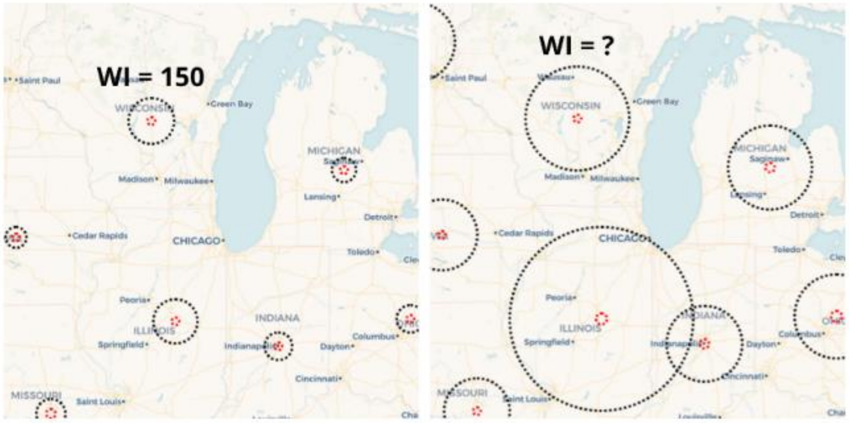


- 300
- 340
- 320
- 280

7. New York (NY) has a black dotted circle with a **diameter** of 430 (as seen on the left image). *

What is the **diameter** of New York (NY)'s black dotted circle on the right?

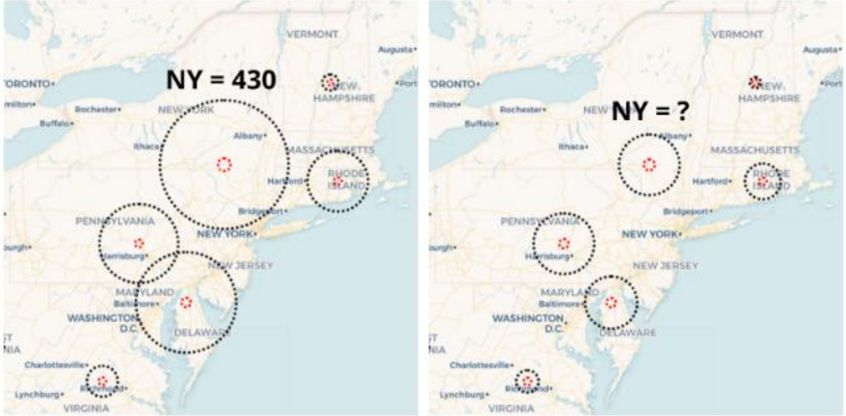


- ◯ 180
- ◯ 200
- ◯ 160
- ◯ 220

8. Texas (TX) has a black dotted square with a **side length** of 620 (as seen on the left image). *

What is the **side length** of Texas (TX)'s black dotted square on the right?

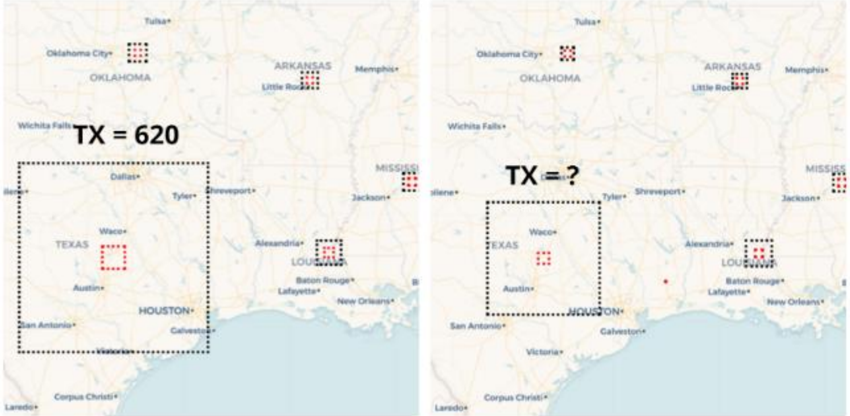


- ◯ 330
- ◯ 350
- ◯ 400
- ◯ 370

9. Serbia has a black dotted square with a **side length** of 120 (as seen on the left image). *

What is the **side length** of Serbia's black dotted square on the right?

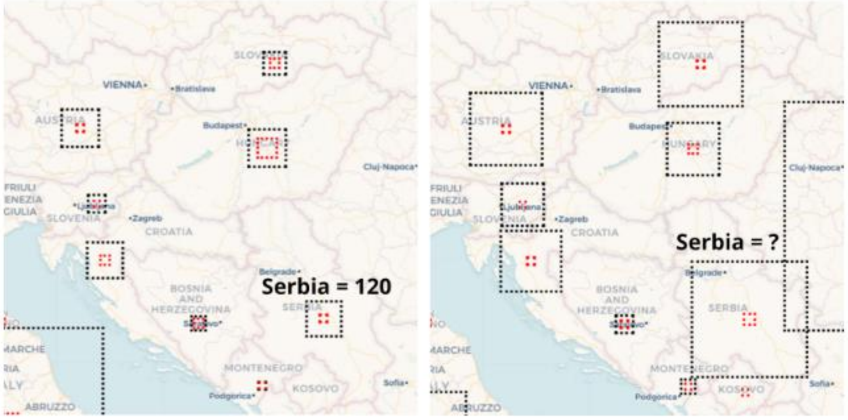


- 400
- 360
- 380
- 420

Section 4 of 9

## Circumference and Perimeter Tasks

Using only the visual information on the maps, please estimate (by eye) the relative sizes of the **black dotted shapes**. Note: the values are arbitrary, so no outside information will be useful.

Definitions:

Circumference of a Circle - the linear distance around the circle (in other words, if a circle is opened to form a straight line, then the length of that line will be the circle's circumference)
Perimeter of a Square - the sum of all 4 side lengths

10. Tunisia has a black dotted circle with a **circumference** of 140. *

What is the **circumference** of Pakistan's black dotted circle?

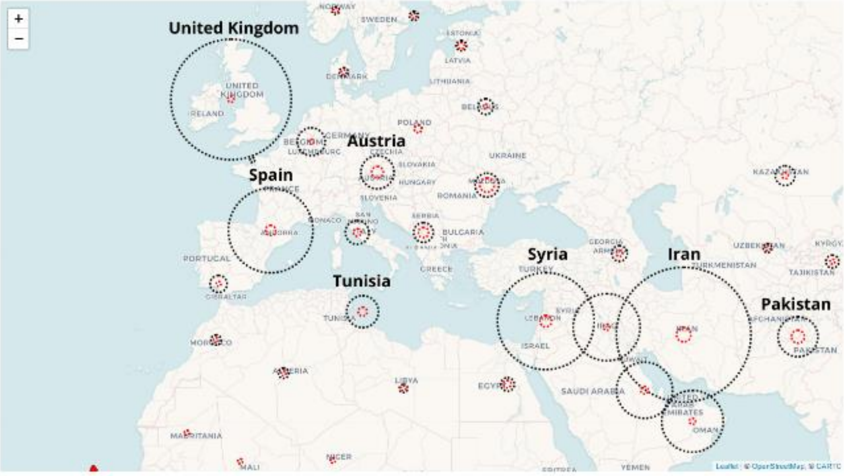


- 160
- 170
- 180
- 190

11. Iran has a black dotted circle with a **circumference** of 630. *

What is the **circumference** of Austria's black dotted circle?

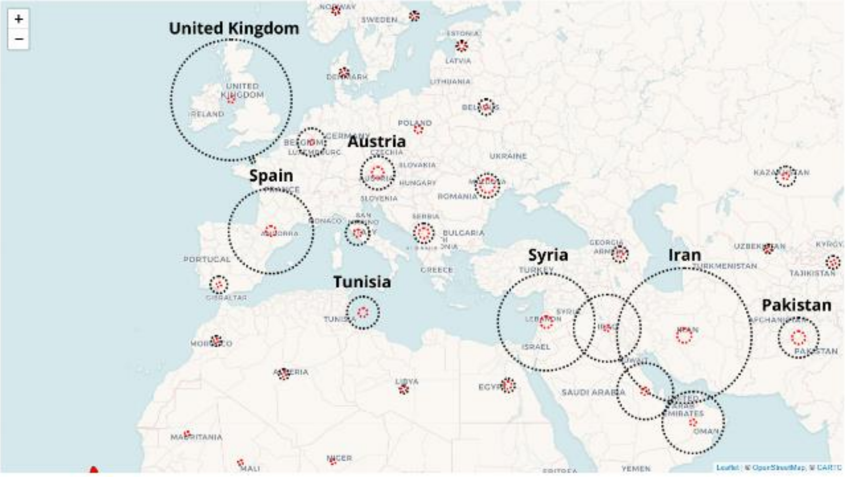


- 200
- 180
- 160
- 140

12. Arizona (D: AZ) has a black dotted square with a **perimeter** of 230. *

What is the **perimeter** of Oklahoma (G: OK)'s black dotted square?

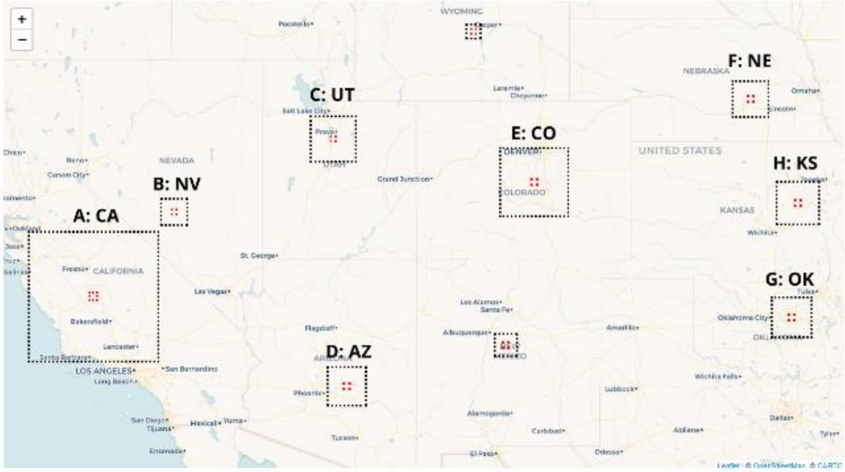


- 220
- 240
- 260
- 280

13. Kansas (H: KS) has a black dotted square with a **perimeter** of 250. *

What is the **perimeter** of Colorado (E: CO)'s black dotted square?

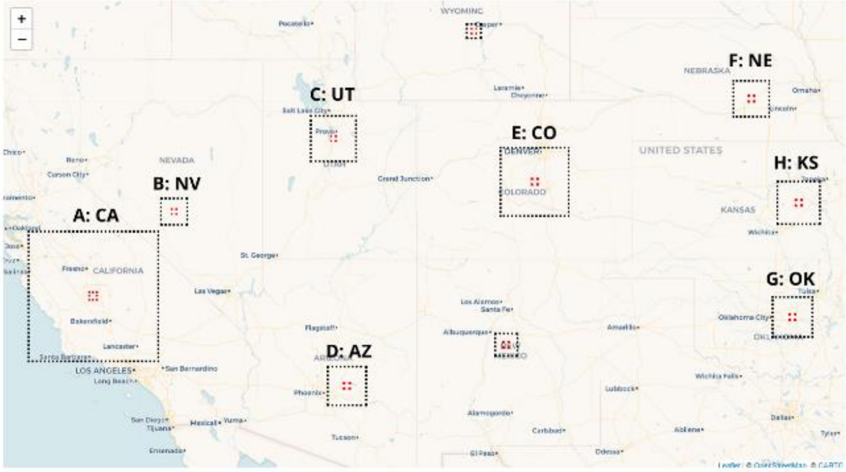


- 380
- 400
- 420
- 440

14. Rhode Island (RI) has a black dotted circle with a **circumference** of 640 (as seen on the left image). *

What is the **circumference** of Rhode Island (RI)'s black dotted circle on the right?

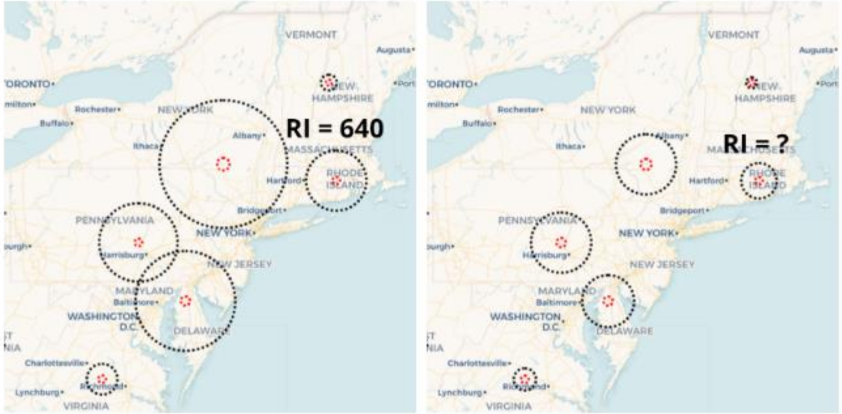


- 380
- 400
- 440
- 360

15. Illinois (IL) has a black dotted circle with a **circumference** of 550 (as seen on the left image). *

What is the **circumference** of Illinois (IL)'s black dotted circle on the right?

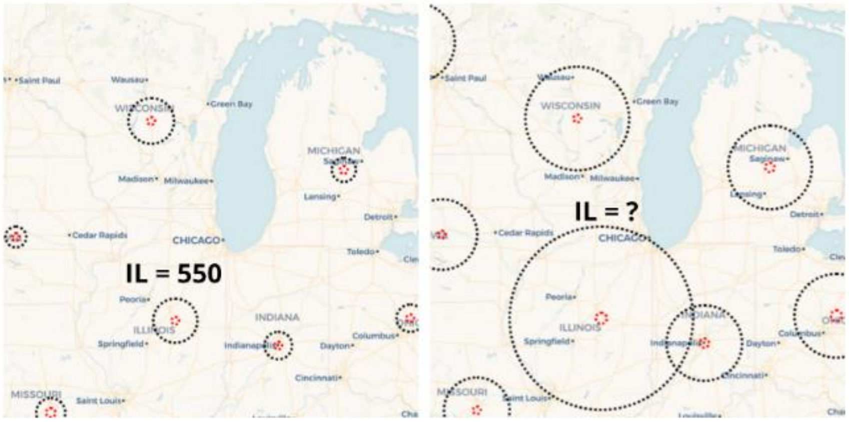


- 1900
- 1800
- 1700
- 2000

16. Tennessee (TN) has a black dotted square with a **perimeter** of 360 (as seen on the left image). *

What is the **perimeter** of Tennessee (TN)'s black dotted square on the right?

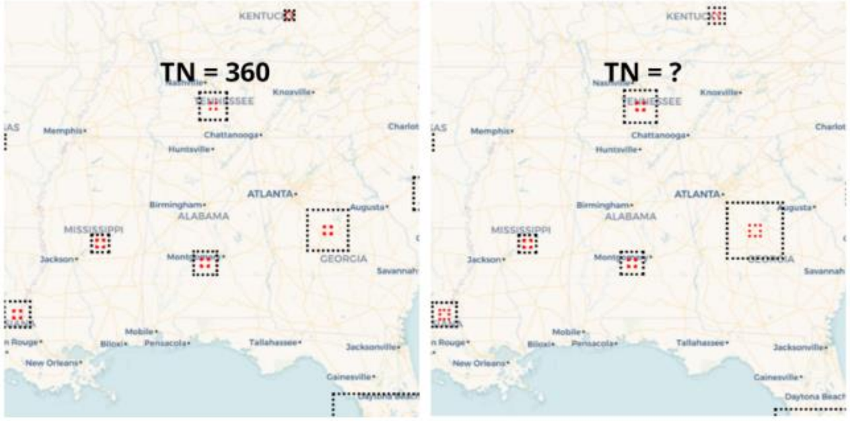


- 400
- 440
- 420
- 460

17. Italy has a black dotted square with a **perimeter** of 2660 (as seen on the left image). *

What is the **perimeter** of Italy's black dotted square on the right?

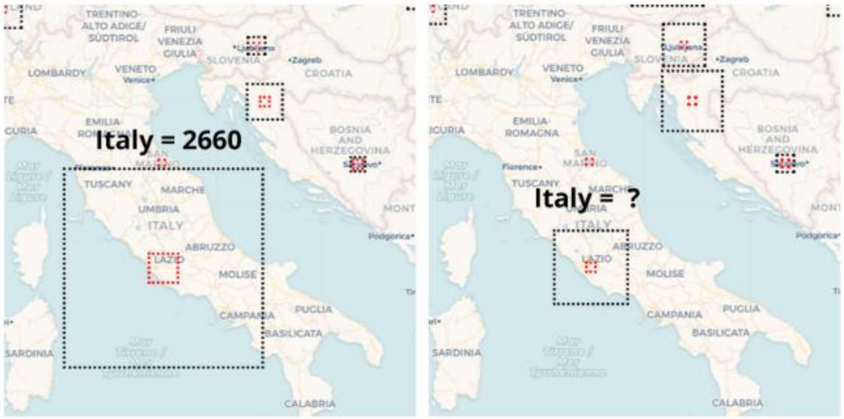


- 1200
- 1000
- 1300
- 900

## Area Tasks

Using only the visual information on the maps, please estimate (by eye) the relative sizes of the **black dotted shapes**. Note: the values are arbitrary, so no outside information will be useful.

Definition:

Area of a shape - the internal region bounded by the shape (in other words, the surface that would be covered if the object were shaded in)

18. Texas (A: TX) has a black dotted circle with an **area** of 3800. *

What is the **area** of Florida (G: FL)'s black dotted circle?

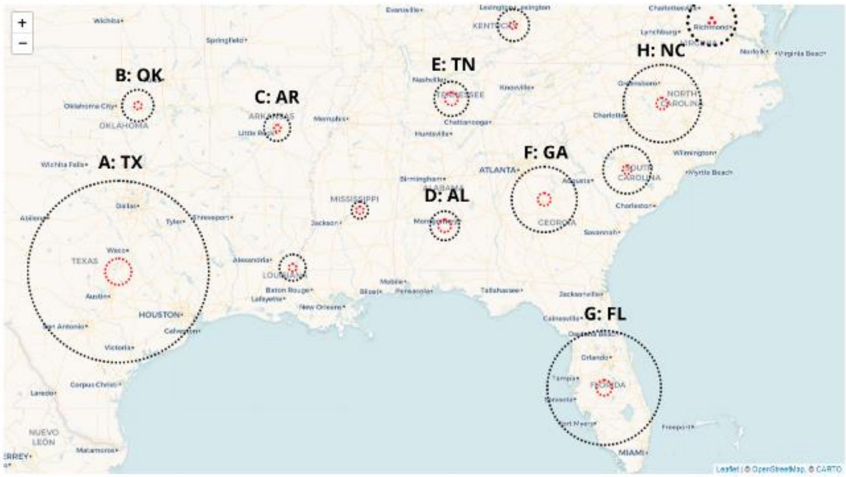


- 1700
- 1300
- 1500
- 1900

19. Georgia (F: GA) has a black dotted circle with an **area** of 520. *

What is the **area** of North Carolina (H: NC)'s black dotted circle?

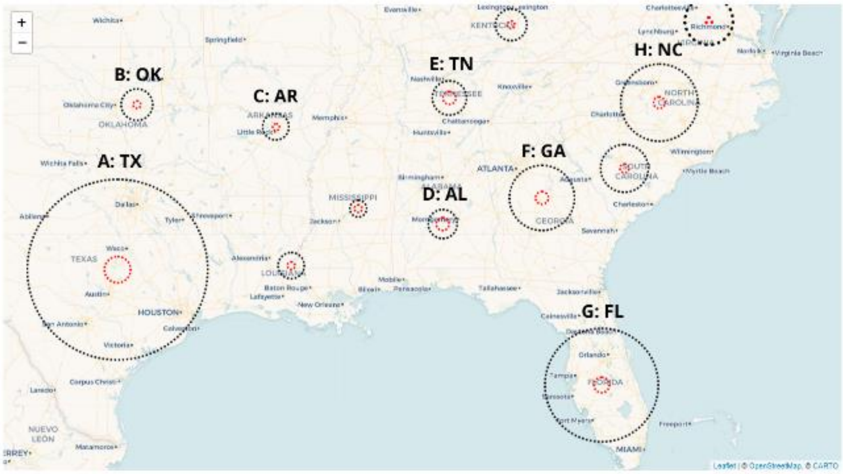


- 680
- 720
- 700
- 740

20. Wisconsin (D: WI) has a black dotted square with an **area** of 200. *

What is the **area** of Kentucky (G: KY)'s black dotted square?

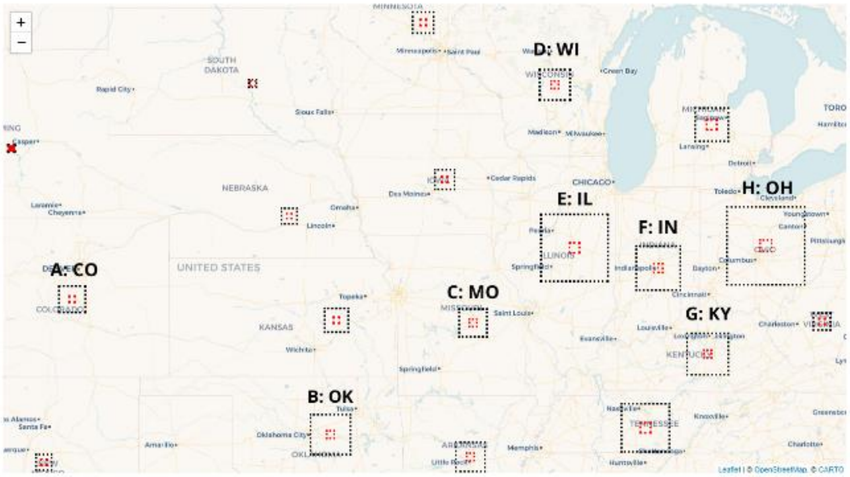


- 360
- 380
- 400
- 420

21. Indiana (F: IN) has a black dotted square with an **area** of 420. *

What is the **area** of Oklahoma (B: OK)'s black dotted square?

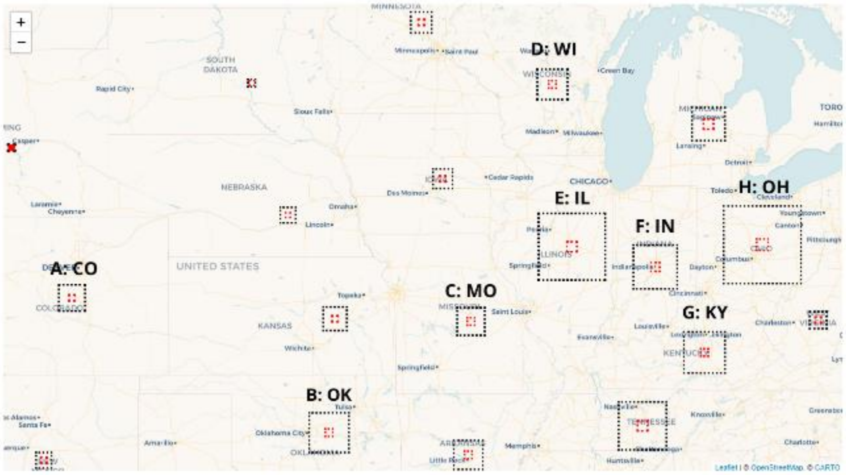


- 380
- 360
- 400
- 420

22. Pennsylvania (PA) has a black dotted circle with an **area** of 2000 (as seen on the left image). *

What is the **area** of Pennsylvania (PA)'s black dotted circle on the right?

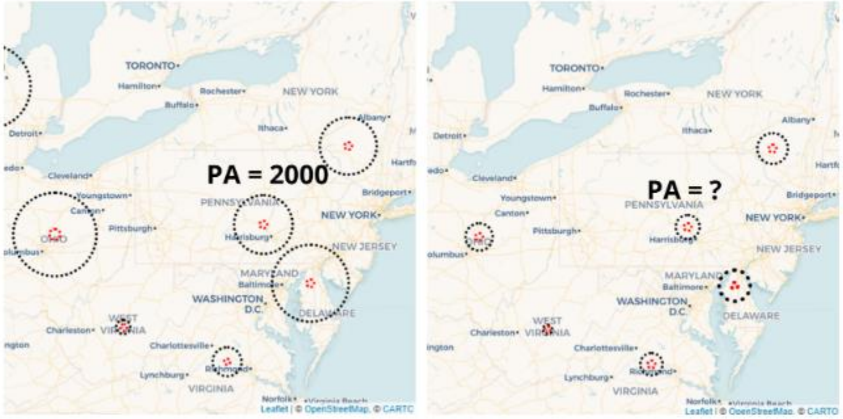


- 300
- 320
- 400
- 360

23. Michigan (MI) has a black dotted circle with an **area** of 350 (as seen on the left image). *

What is the **area** of Michigan (MI)'s black dotted circle on the right?

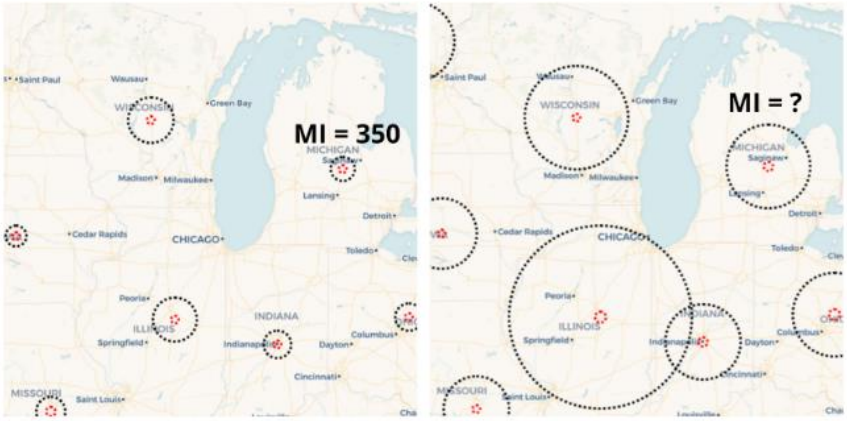


- 4000
- 4200
- 3600
- 4400

24. Austria has a black dotted square with an **area** of 1000 (as seen on the left image). *

What is the **area** of Austria's black dotted square on the right?

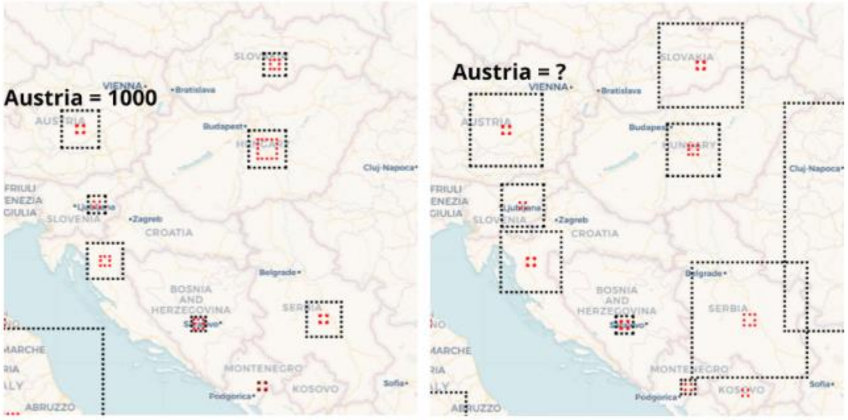


- 3600
- 3800
- 4400
- 4200

25. Georgia (GA) has a black dotted square with an **area** of 2200 (as seen on the left image). *

What is the **area** of Georgia (GA)'s black dotted square on the right?

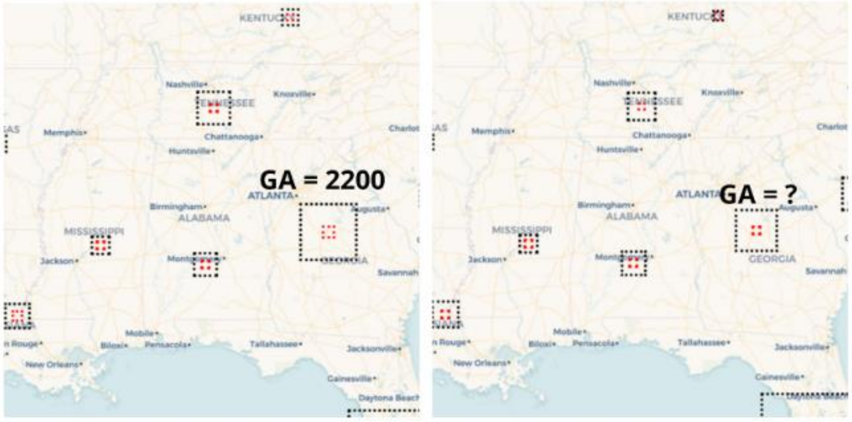


- ◯ 1400
- ◯ 1200
- ◯ 1000
- ◯ 800

Section 6 of 9

## General Questions pt1

Description (optional)

Across all the tasks, for which **shape** did you find it easiest to estimate the relative size? *

- ◯ Circles
- ◯ Squares
- ◯ Same difficulty

Across all the tasks, for which **measurement** did you find it easiest to estimate the relative size? *

- ◯ Diameter/Side Length
- ◯ Circumference/Perimeter
- ◯ Area
- ◯ Same difficulty

Section 7 of 9

General Questions pt2

Description (optional)

Just by looks, which **center circle** looks bigger? *

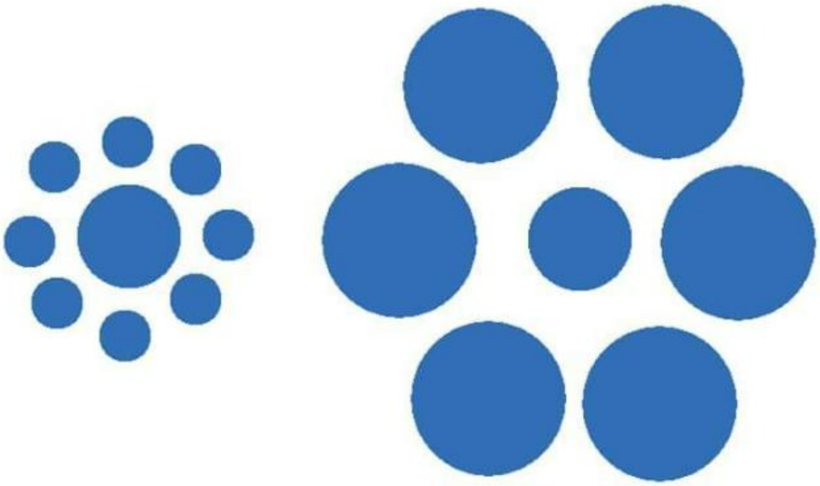

- Left
- Right
- Same Size

Just by looks, which **center square** looks bigger? *

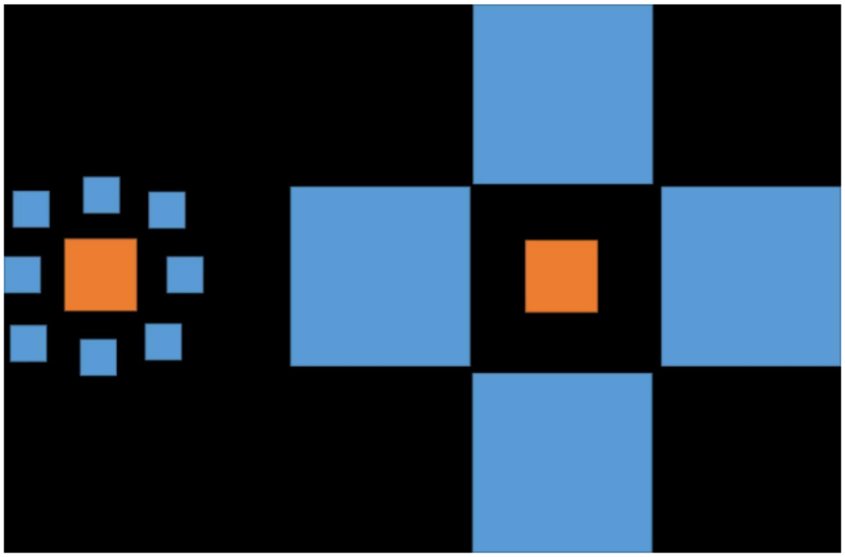

- ◯ Left
- ◯ Right
- ◯ Same Size

Section 8 of 9

## Demographics

Description (optional)

What is your age range? *

- ◯ 18-20
- ◯ 21-30
- ◯ 31-40
- ◯ 41-50
- ◯ 51-60
- ◯ 61+
- ◯ Prefer not to answer

What is your gender? *

- ◯ Male
- ◯ Female
- ◯ Prefer not to answer

What is the highest degree or level of school you have completed or are currently enrolled in? *

- Less than High School
- High School or Equivalent
- Associate degree
- Bachelors degree
- Masters or Professional
- Terminal degree (PhD/MD/JD)
- Prefer not to answer

Additional Comments

Long answer text

After section 8 Continue to next section

Section 9 of 9

Thank you! Please see the completion code below

COMPL3T3DCORONAV!Z
